# Supplementary material for: User-Friendly Game-Theoretic Modeling and Analysis of Multi-Modal Transportation Systems
Source: arXiv:2502.04155 source file (2025-02-06)
Supplement: Supplementary file 1 [file appendix.tex]

\section{Proofs}
\label{sec:appendix}
